# Supplementary material for: AMAE: Adaptation of Pre-Trained Masked Autoencoder for Dual-Distribution Anomaly Detection in Chest X-Rays
Source: arXiv:2307.12721 source file (2023-07-28)
Supplement: Supplementary file 1 [file paper-1205_appendix.tex]

\appendix

\section{Ablation Study} 
\label{sec:ablation}
\vspace{-2mm}
\begin{table}
\centering
\caption{\textbf{Ablations for the number of generated masks $L$ and making ratio} used for the adaptation $\AMAE$-\textbf{Stage 2} ($\mathcal{A}_{inter}$) on the RSNA dataset.}
\resizebox{0.5\linewidth}{!}{
\begin{tabular}{@{}l|cc@{}}
\hline
\multirow{2}{*}{\textbf{Baselines}}                   & \multicolumn{2}{c}{ \textbf{Different Masking Ratio}}  \\ \cline{2-3}
                     & \multicolumn{1}{c}{AUC$\%$} &  AP$\%$                            \\ \hline
50$\%$                & \multicolumn{1}{c}{$90.2$}        & $89.1$ \\
$\cellcolor[HTML]{FFD480}75\%$                 & {$\cellcolor[HTML]{FFD480}91.4$}         & $\cellcolor[HTML]{FFD480}91.7$ \\
90$\%$                         & \multicolumn{1}{c}{$89.2$}        & $88.3$ \\
%MSN~\cite{assran2022masked} &  \multicolumn{1}{c|}{$97.8$\std{$0.6$}}        & $97.9$\std{$0.8$} \\
 \hline
\multirow{2}{*}{}                   & \multicolumn{2}{c}{\textbf{Number of generated masks $L$}}  \\ \cline{2-3}
                     & \multicolumn{1}{c}{AUC$\%$} &  AP$\%$                             \\ \hline
$L=1$                & \multicolumn{1}{c}{$88.5$}      & $87.4$ \\
$\cellcolor[HTML]{FFD480}L=2$                 & \multicolumn{1}{c}{$\cellcolor[HTML]{FFD480}91.4$}      & $\cellcolor[HTML]{FFD480}91.7$ \\
$L=3$                & \multicolumn{1}{c}{$91.3$}      & $91.6$ \\
\hline
\end{tabular}
}
\label{tab:masking}
\end{table}
%\vspace{-1.5em}
\vspace{-2mm}

\newpage
\section{Implementation Details \& Inference Time}
\label{sec:app_implementation_details}
%\noindent

\begin{figure}
    \frame{\includegraphics[width=0.5\textwidth]{MICCAI23_MAE/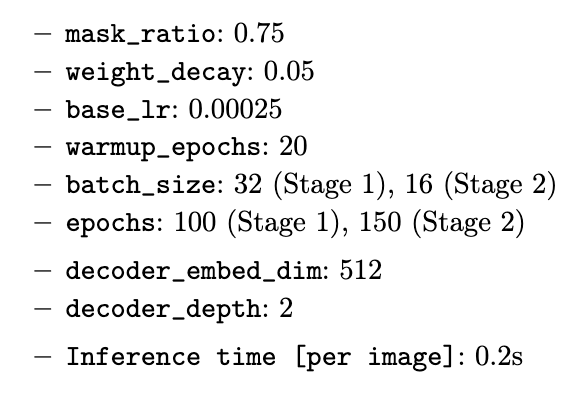}}
    \caption{\textbf{Implementation details and inference time}. Implementation details of the MAE adapted under our $\AMAE$ framework. We tested the running time for each test image of the RSNA test set on a GeForce RTX 2080 Ti GPU for \textbf{$\AMAE$-Stage 2} ($\mathcal{A}_{inter}$). Only 25\% of the tokens are fed to MAE encoders of both modules. } \label{fig3}
\end{figure}

% \Thomas{
% The spatial tokens of the pre-trained and frozen model are fed to object discovery methods, i.e. LOST \cite{simeoni2021localizing}, TokenCut \cite{wang2022self} and DSM \cite{melas2022deep}. The commonly adopted CorLoc metric is reported on standard single object discovery datasets: VOC07, VOC12 and COCO20k. ``The Correct Localization (CorLoc) metric, i.e., the percentage of correct boxes, where a predicted box is considered correct if it has an intersection over union (IoU) score superior to 0.5 with one of the labeled object bounding boxes.'' Sentence from LOST \cite{simeoni2021localizing}.
% }
